# Supplementary material for: Development of an automated millifluidic platform and data-analysis pipeline for rapid electrochemical corrosion measurements: a pH study on Zn-Ni
Source: arXiv:2204.06094 source file (2022-04-01)
Supplement: Supplementary file 1 [file SDC_Dev_ZnNi__SI__1_.pdf]

# Supplementary Information: Development of an automated millifluidic platform and data-analysis pipeline for rapid electrochemical corrosion measurements: a pH study on Zn-Ni

Howie Joress[a], Brian DeCost[a], Najlaa Hassan[a,b], Trevor M. Braun[c], Justin M. Gorham[a], Jason Hattrick-Simpers[a]

[a] *Materials Measurment Science Division National Institute of Standards and Technology Gaithersburg MD 20889 USA*
[b] *University of Wisconsin Madison*
[c] *Materials Science and Engineering Division National Institute of Standards and Technology Gaithersburg MD 20899*

*Email address:* howie.joress@nist.gov (Howie Joress)

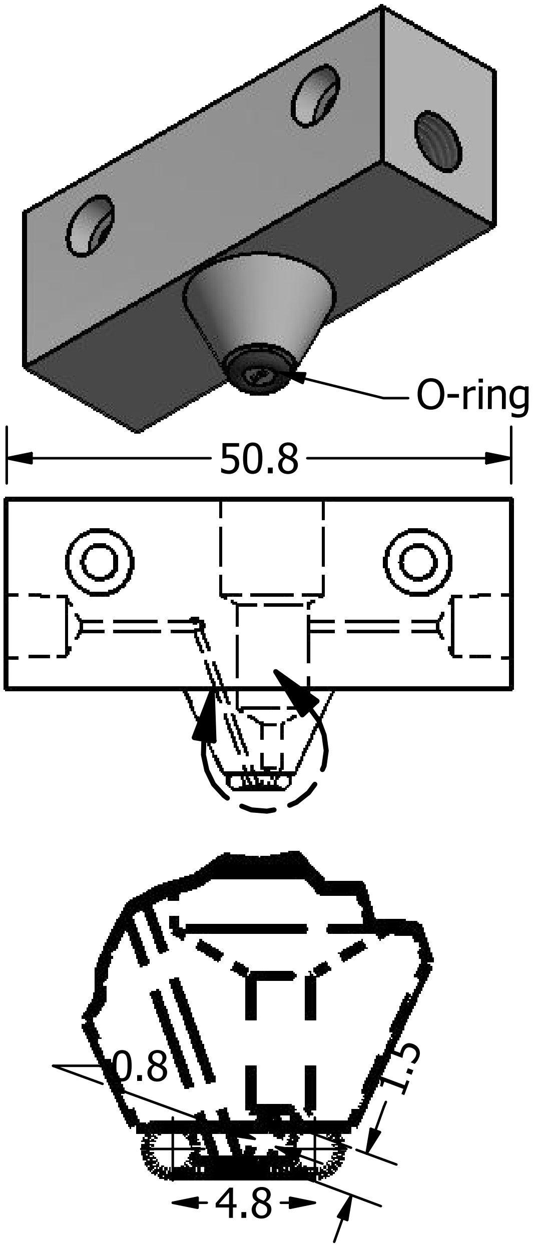


Fig. S1: Technical drawings of the SDC head to scale. (a) is an isometric sketch of the cell head showing the O-ring. (b) is a view of the cell head showing the internal components. (c) is a 3:1 view of the tip of the cell head showing inlet and outlet to the probe volume.

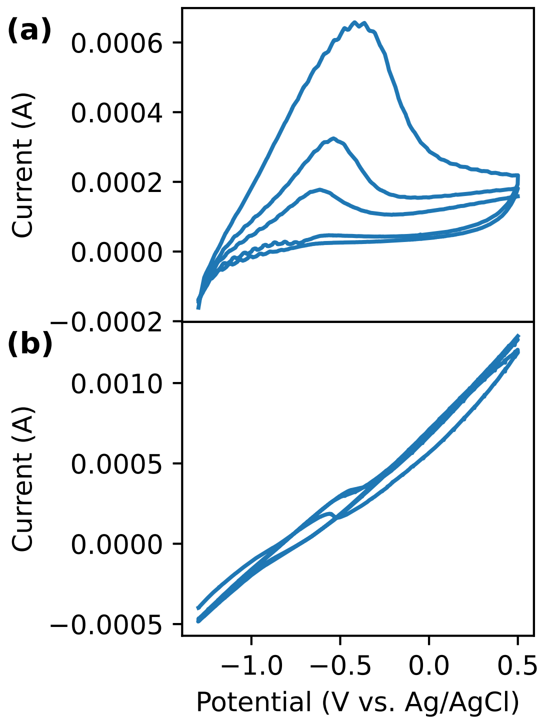


Fig. S2: Two cyclic voltamagrams at different pHs: 12.4 and 10.5 for top and bottom respectively. For the lower curve the resistance drop through the cell dominates the voltamagram making it uninterpretable.

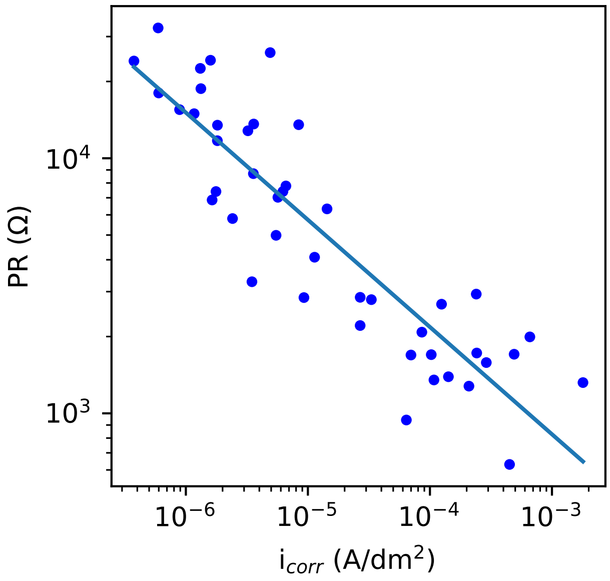


Fig. S3: Plot showing comparing the polarization resistance and the $i_{corr}$ from the LPR and Tafel measurements respectively. $R^2$ of the regression is 0.78.

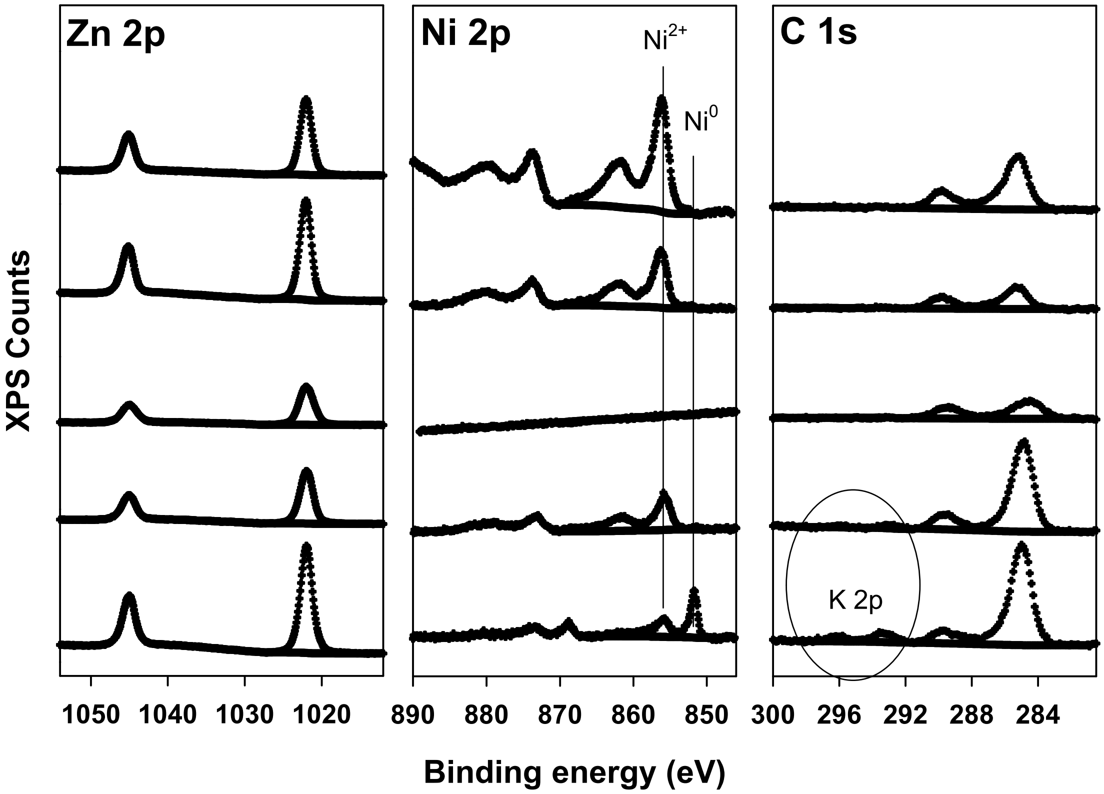


Fig. S4: Plots showing the raw XPS data with associated fitted background. Plots show data offset for clarity with every other point shown and starting from low pH at the top to high pH at the bottom. The native surface is not shown. The left plot shows the Zn edge. The center plot shows the Ni edge and the peak shift associated with change of valency, and the right plot shows the carbon edge as well as some background potassium from remnant crystalized electrolyte.
